# Supplementary material for: A new provably stable weighted state redistribution algorithm
Source: arXiv:2308.16332 source file (2024-04-02)
Supplement: Supplementary file 1 [file supplementary_materials.pdf]

# SUPPLEMENTARY MATERIALS: A NEW PROVABLY STABLE WEIGHTED STATE REDISTRIBUTION ALGORITHM

MARSHA BERGER* AND ANDREW GIULIANI†

This supplementary material provides a proof that SRD on the 1D model problem is total variation diminishing (TVD). We provide monotonicity proofs for central merging $2 \times 2$ case Property 4 (Sec. SM2.1), the $3 \times 3$ case Property 5 (Sec. SM2.2), and an additional configuration using normal merging with an overlap count of 3 (Sec. SM3), giving Property 6. Equations and figures referenced in the main document retain the same numbering here.

## SM1. SRD is TVD in 1D.

First we will prove

**Theorem:** Consider the model problem in one space dimension with one small cell, the first order upwind method $u_j^{n+1} = u_j^n - \lambda(u_j^n - u_{j-1}^n)$, and merging left with SRD using the new monotone weights for $0 \leq \lambda \leq 1$, $\alpha_{\text{target}} = 1$, and $w_{\text{-}1,\text{-}1} = \alpha$. The scheme is total variation diminishing (TVD), i.e. $\sum_i |U_i - U_{i-1}|$ decreases in time, when used with pre-merging (4.1) applied to the initial conditions.

*Remark:* Without pre-merging there are overshoots and SRD is not TVD. It is unintuitive (at least to us) that a single step of merging applied to the initial conditions, fixes this.

We show the scheme is TVD in three steps. First we show that the pre-merging step is TVD. Next we show that going from $Q^{n-1}$ to $Q^n$ is TVD, for $n \geq 1$. Finally we show that the step from $Q^{n-1}$ to $U^n$ is TVD, $n \geq 1$. We use the notation $U^0 = SRD(U^{init})$, and we introduce the variable $\widehat{Q}^{\text{-}1}$, which is the merging neighborhood averages during this pre-merging step "at time -1, i.e. before time 0", and should not be confused with an inverse.

We only need to look at the cells affected by SRD. Recall that cell -1 and cell -2 are both regular, so their merging neighborhood averages are $\widehat{Q}^{\text{-}1}_{\text{-}2} = U^{init}_{\text{-}2}$, and $\widehat{Q}^{\text{-}1}_{\text{-}1} = U^{init}_{\text{-}1}$ come directly from the initial conditions now. For this pre-merging step, the neighborhood average on cell 0 is $\widehat{Q}^{\text{-}1}_0 = \gamma U^{init}_{\text{-}1} + (1-\gamma) U^{init}_0$, where $\gamma =$

*Flatiron Institute, New York City, New York (mberger@flatironinstitute.org). Also Professor Emeritus, Courant Institute, New York University
†Flatiron Institute, New York City, New York (agiuliani@flatironinstitute.org).



*This manuscript is for review purposes only.*

$(1-w_{-1,-1})/(\alpha+1-w_{-1,-1})$. We have

$$T_1 = \sum_{i\le -3} (\widehat{Q}^{-1}_i - \widehat{Q}^{-1}_{i+1}) \le \sum_{i\le -3} |U^{init}_i - U^{init}_{i+1}|$$

$$T_2 = \widehat{Q}^{-1}_{-2} - \widehat{Q}^{-1}_{-1} = U^{init}_{-2} - U^{init}_{-1}$$

$$T_3 = \widehat{Q}^{-1}_{-1} - \widehat{Q}^{-1}_{0} = U^{init}_{-1} - \gamma U^{init}_{-1} - (1-\gamma)U^{init}_0 = (1-\gamma)(U^{init}_{-1} - U^{init}_0)$$

$$\begin{aligned} T_4 = \widehat{Q}^{-1}_{0} - \widehat{Q}^{-1}_{1} &= \gamma U^{init}_{-1} + (1-\gamma)U^{init}_0 - U^{init}_1 \\ &= \gamma(U^{init}_{-1} - U^{init}_0) + (U^{init}_0 - U^{init}_1) \end{aligned}$$

$$T_5 = \sum_{i\ge 1} (\widehat{Q}^{-1}_i - \widehat{Q}^{-1}_{i+1}) \le \sum_{i\ge 1} |U^{init}_i - U^{init}_{i+1}|$$

Since we have $0 \le w_{-1,-1} \le 1$, all the multipliers are positive. Applying the triangle inequality and summing the estimates shows that the pre-merging step $TV(Q^{-1}) \le TV(U^{init})$ is TVD.

Next we show that $TV(\widehat{Q}^{n+1}) \le TV(\widehat{Q}^n)$. We can write $TV(\widehat{Q}^{n+1})$ as a sum of the following terms:

$$T_1 = \sum_{i\le -3} \widehat{Q}^{n+1}_i - \widehat{Q}^{n+1}_{i+1} = \sum_{i\le -3} (1-\lambda)(\widehat{Q}^n_i - Q^n_{i+1}) + \lambda \sum (\widehat{Q}^n_{i-1} - \widehat{Q}^n_i)$$

$$\begin{aligned} T_2 = \widehat{Q}^{n+1}_{-2} - \widehat{Q}^{n+1}_{-1} = &(1-\lambda)(1-w_{-1,-1})(\widehat{Q}_{-1} - \widehat{Q}_0) + (1-\lambda)(\widehat{Q}^n_{-2} - \widehat{Q}^n_{-1}) + \\ &\lambda(\widehat{Q}^n_{-3} - \widehat{Q}^n_{-2}) \end{aligned}$$

$$\begin{aligned} T_3 = \widehat{Q}^{n+1}_{-1} - \widehat{Q}^{n+1}_{0} = &\lambda\left(1 - \frac{1-w_{-1,-1}}{\widehat{V}_0}\right)(\widehat{Q}^n_{-2} - \widehat{Q}^n_{-1}) + \\ &\left[(1-w_{-1,-1})\lambda + w_{-1,-1} - \frac{(\lambda+w_{-1,-1})(1-w_{-1,-1}) + \lambda w^2_{-1,-1}}{\widehat{V}_0}\right](\widehat{Q}^n_{-1} - \widehat{Q}^n_0) \end{aligned}$$

$$\begin{aligned} T_4 = \widehat{Q}^{n+1}_{0} - \widehat{Q}^{n+1}_{1} = &(1-\lambda)(\widehat{Q}^n_0 - \widehat{Q}^n_1) + \frac{\lambda + w_{-1,-1}(1-w_{-1,-1})(1-\lambda)}{\widehat{V}_0}(\widehat{Q}^n_{-1} - \widehat{Q}^n_0) \\ &+ \frac{\lambda(1-w_{-1,-1})}{\widehat{V}_0}(\widehat{Q}^n_{-2} - \widehat{Q}^n_{-1}) \end{aligned}$$

$$T_5 = \sum_{i\ge 1} \widehat{Q}^{n+1}_i - \widehat{Q}^{n+1}_{i+1} = \sum_{i\ge 1} (1-\lambda)(\widehat{Q}^n_i - \widehat{Q}^n_{i+1}) + \lambda \sum (\widehat{Q}^n_{i-1} - \widehat{Q}^n_i)$$

where $\widehat{V}_0 = 1 + \alpha - w_{-1,-1}$ is the weighted volume. Assume now that $0 \le w_{-1,-1} \le \alpha$ and using $0 \le \lambda \le 1$ gives the estimates

$$|T_2| \le (1-\lambda)(1-w_{-1,-1})|\widehat{Q}^n_{-1} - \widehat{Q}^n_0| + (1-\lambda)|\widehat{Q}^n_{-2} - \widehat{Q}^n_{-1}| + \lambda|\widehat{Q}^n_{-3} - \widehat{Q}^n_{-2}|$$

$$\begin{aligned} |T_3| \le &\lambda\left(1 - \frac{1-w_{-1,-1}}{\widehat{V}_0}\right)|\widehat{Q}^n_{-2} - \widehat{Q}^n_{-1}| \\ &+ \left[(1-w_{-1,-1})\lambda + w_{-1,-1} - \frac{(\lambda+w_{-1,-1})(1-w_{-1,-1}) + \lambda w^2_{-1,-1}}{\widehat{V}_0}\right]|\widehat{Q}^n_{-1} - \widehat{Q}^n_0| \end{aligned}$$

$$\begin{aligned} |T_4| \le &(1-\lambda)|\widehat{Q}^n_0 - \widehat{Q}^n_1| + \frac{\lambda + w_{-1,-1}(1-w_{-1,-1})(1-\lambda)}{\widehat{V}_0}|\widehat{Q}^n_{-1} - \widehat{Q}^n_0| \\ &+ \frac{\lambda(1-w_{-1,-1})}{\widehat{V}_0}|\widehat{Q}^n_{-1} - \widehat{Q}^n_{-2}| \end{aligned}$$

Summing, we have

$$|T_2| + |T_3| + |T_4| \le \lambda|\widehat{Q}^n_{\text{-}3} - \widehat{Q}^n_{\text{-}2}| + |\widehat{Q}^n_{\text{-}2} - \widehat{Q}^n_{\text{-}1}| + |\widehat{Q}^n_{\text{-}1} - \widehat{Q}^n_0| + (1-\lambda)|\widehat{Q}^n_0 - \widehat{Q}^n_1|$$

which results in $TV(\widehat{Q}^{n+1}) \le TV(\widehat{Q}^n)$ after accounting for telescoping terms.

Finally, we check that the total variation at the final step is diminishing

$$TV(U^{n+1}) \le TV(\widehat{Q}^n) \quad \text{for } n \ge 0,$$

which completes a full step. We have:

$$\begin{aligned}
T_1 &= \sum_{i\le -3} (U_i^{n+1} - U_{i+1}^{n+1}) \le \sum_{i\le -3} |\widehat{Q}^n_i - \widehat{Q}^n_{i+1}| \\
T_2 &= U^{n+1}_{\text{-}2} - U^{n+1}_{\text{-}1} = (\widehat{Q}^n_{\text{-}2} - \widehat{Q}^n_{\text{-}1}) + (1 - w_{\text{-}1,\text{-}1})(\widehat{Q}^n_{\text{-}1} - \widehat{Q}^n_0) \\
&\le |\widehat{Q}^n_{\text{-}2} - \widehat{Q}^n_{\text{-}1}| + (1 - w_{\text{-}1,\text{-}1})|\widehat{Q}^n_{\text{-}1} - \widehat{Q}^n_0| \\
T_3 &= U^{n+1}_{\text{-}1} - U^{n+1}_0 = w_{\text{-}1,\text{-}1}\widehat{Q}^n_{\text{-}1} + (1 - w_{\text{-}1,\text{-}1})\widehat{Q}^n_0 - \widehat{Q}^n_0 \le w_{\text{-}1,\text{-}1}|\widehat{Q}^n_{\text{-}1} - \widehat{Q}^n_0| \\
T_4 &= U^{n+1}_0 - U^{n+1}_1 \le |\widehat{Q}^n_0 - \widehat{Q}^n_1| \\
T_5 &= \sum_{i\ge 1}(U_i^{n+1} - U_{i+1}^{n+1}) \le \sum_{i\ge 1} |\widehat{Q}^n_i - \widehat{Q}^n_{i+1}|
\end{aligned}$$

A similar proof holds for merging right instead of left. ■

**SM2. Central Merging, $45^\circ$ Planar Boundary.** Next we apply the general formula (4.2) to central merging instead of normal merging. This involves a change in the composition of the set $M_0$ of cells contributing to $Q_0$'s neighborhood. Figure SM1 illustrates the two possibilities.

The advection velocity can now be taken to be $\mathbf{a} = [1, 1]$, the maximum stable time step satisfies $\Delta t\, 2/h = 1$, $l = l_{0,1} = l_{2,0}$, and $0 \le l \le 1$. The parameters are

$$\begin{aligned}
\alpha_0, \alpha_4, \alpha_6 &= \frac{1}{2}l^2, & \alpha_1, \alpha_2 &= 1 - \frac{1}{2}(1-l)^2 \\
\lambda_0, \lambda_6, \lambda_4, \lambda_{0,1}, \lambda_{2,0} &= \Delta t \frac{l}{h}, & \lambda_{5,2}, \lambda_{1,5} &= \frac{\Delta t}{h} \\
\lambda_1, \lambda_2 &= \Delta t \frac{1+l}{h}, & \lambda_5 &= \Delta t \frac{2}{h}.
\end{aligned} \tag{SM2.1}$$

**SM2.1. Property 4.** Central merging in the 2 by 2 case using the weights of (4.2) results in monotone weights with the full CFL.

First we adapt the general formula (A.7) to the $2 \times 2$ central merging case, where

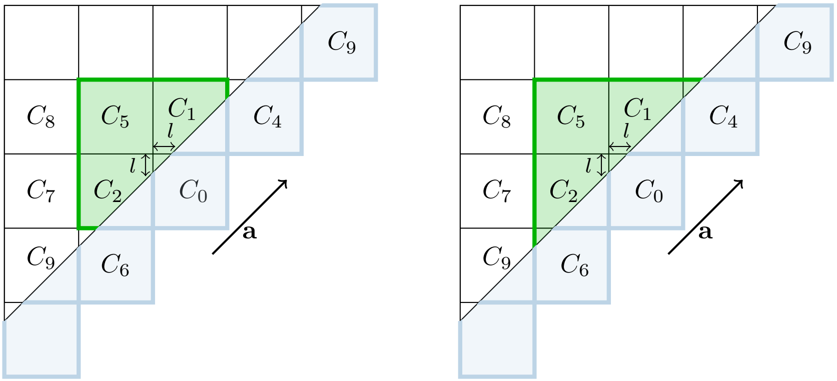


FIG. SM1. *Notation for the two possible merging configurations in 2D with SRD using central merging (green cells) and flow parallel to a planar boundary. Left and right show respectively* $2 \times 2$ *and* $3 \times 3$ *central merging.*

$M_0 = \{0, 1, 2, 5\}$, obtaining

$$
\begin{aligned}
\frac{\widehat{V}_0}{h^2}\widehat{Q}_0^n = \Big( &(\alpha_0 - \lambda_0) + w_{1,0}^2(\alpha_1 - \lambda_1) + w_{2,0}^2(\alpha_2 - \lambda_2) + w_{5,0}^2(\alpha_5 - \lambda_5) \\
&+ w_{2,0}\lambda_{0,2} + w_{1,0}\lambda_{1,0} + w_{1,0}w_{5,0}\lambda_{1,5} + w_{5,0}w_{2,0}\lambda_{5,2}\Big)\widehat{Q}_0^{n-1} \\
&+ (w_{1,0} - w_{1,0}^2)(\alpha_1 - \lambda_1)\,\widetilde{Q}_1^{n-1} \\
&+ [\lambda_{0,2}\,(1 - w_{2,0}) + (w_{2,0} - w_{2,0}^2)(\alpha_2 - \lambda_2) + w_{5,0}\lambda_{5,2}\,(1 - w_{2,0})]\,\widetilde{Q}_2^{n-1} \\
&+ [w_{1,0}\lambda_{1,5}(1 - w_{5,0}) + (w_{5,0} - w_{5,0}^2)(\alpha_5 - \lambda_5)]\widetilde{Q}_5^{n-1} \\
&+ w_{2,0}\lambda_{2,6}\,\widetilde{Q}_6^{n-1} + w_{2,0}\lambda_{2,7}\,\widetilde{Q}_7^{n-1} + w_{5,0}\lambda_{5,8}\,\widetilde{Q}_8^{n-1}.
\end{aligned}
\tag{SM2.2}
$$

The only multiplier that is possibly negative corresponds to the $\widehat{Q}_0^{n-1}$ term, caused by $\alpha_0 - \lambda_0$. The other multipliers are clearly non-negative because $0 \le w_{5,0}, w_{2,0}, w_{1,0} \le 1$, and because we are using monotonicity on the unmerged cut cells (Property 2). It follows that $\alpha_5 - \lambda_5 \ge 0$, $\alpha_1 - \lambda_1 \ge 0$, and $\alpha_2 - \lambda_2 \ge 0$. We only have two weights that are free to specify: $w_{1,0}, w_{5,0}$, since for symmetry we require $w_{2,0} = w_{1,0}$. Substituting in (SM2.2) and using $\lambda_{5,1} = \lambda_{1,5}$, $\lambda_{1,0} = \lambda_{0,1}$, we obtain

$$
\begin{aligned}
\frac{\widehat{V}_0}{h^2}\widehat{Q}_0^n = &\left((l - l^2)w_{1,0}^2 + w_{1,0}(l + w_{5,0}) + \frac{1}{2}(l^2 - l)\right)\widehat{Q}_0^{n-1} \\
&+ \text{many other clearly non-negative terms}\,.
\end{aligned}
\tag{SM2.3}
$$

Substituting in the monotone weights from (4.2) with $N_1 = N_2 = 3$, $N_5 = 2$, gives $w_{1,0} = w_{2,0} = \frac{1}{2} - \alpha_0$ and $w_{5,0} = 1 - 2\alpha_0$. We need to show positivity of the coefficcient in (SM2.3) for monotonicity. Writing everything as a function of $l$ gives

$$
1/2 + l/4 - 3l^2/4 - l^3 + l^4 + l^5/4 - l^6/4 \ge 0.
$$

An algebraic computation shows this is non-negative on the interval $l \in (0, 1]$. ∎

**SM2.2. Property 5.** There are no symmetric non-trivial weights that result in positive multipliers for $3 \times 3$ central merging, and it is not a monotone scheme.

Adapting (A.7) to the 3 by 3 case, we now have $M_0 = \{0, 1, 2, 4, 5, 6\}$. We obtain

$$\begin{aligned}
\frac{\widehat{V}_0}{h^2}\widehat{Q}_0^n &= \widehat{Q}_0^{n-1}(\alpha_0 - \lambda_0 + w_{1,0}^2(\alpha_1 - \lambda_1) + w_{2,0}^2(\alpha_2 - \lambda_2) + w_{4,0}^2(\alpha_4 - \lambda_4) \\
&\quad + w_{5,0}^2(\alpha_5 - \lambda_5) + w_{6,0}^2(\alpha_6 - \lambda_6) + \lambda_{1,0}w_{1,0} + \lambda_{1,5}w_{5,0}w_{1,0} \\
&\quad + \lambda_{4,1}w_{4,0}w_{1,0} + \lambda_{0,2}w_{2,0} + \lambda_{2,6}w_{2,0}w_{6,0} + \lambda_{5,2}w_{2,0}w_{5,0}) \\
&\quad + \widetilde{Q}_4^{n-1}(w_{4,0} - w_{4,0}^2)(\alpha_4 - \lambda_4) \\
&\quad + \widetilde{Q}_5^{n-1}[(w_{5,0} - w_{5,0}^2)(\alpha_5 - \lambda_5) + \lambda_{1,5}w_{1,0}(1 - w_{5,0})] \\
&\quad + \widetilde{Q}_6^{n-1}[(w_{6,0} - w_{6,0}^2)(\alpha_6 - \lambda_6) + \lambda_{2,6}w_{2,0}(1 - w_{6,0})] \\
&\quad + \widetilde{Q}_1^{n-1}[(w_{1,0} - w_{1,0}^2)(\alpha_1 - \lambda_1) + \lambda_{4,1}w_{4,0}(1 - w_{1,0})] \\
&\quad + \widetilde{Q}_2^{n-1}[(w_{2,0} - w_{2,0}^2)(\alpha_2 - \lambda_2) + \lambda_{5,2}w_{5,0}(1 - w_{2,0}) \\
&\quad - \lambda_{0,2}w_{2,0} + \lambda_{0,2}] + \lambda_{2,7}w_{2,0}\widetilde{Q}_7^{n-1} + \lambda_{5,8}w_{5,0}\widetilde{Q}_8^{n-1} + \lambda_{6,9}w_{6,0}\widetilde{Q}_9^{n-1}.
\end{aligned} \tag{SM2.4}$$

Instead of analyzing the multiplier of $\widehat{Q}_0^{n-1}$ as we did previously, we focus on the problematic term $\widetilde{Q}_4^{n-1}(w_{4,0} - w_{4,0}^2)(\alpha_4 - \lambda_4)$. The cell 4 volume fraction $\alpha_4 = \frac{1}{2}\,l^2$ and $\lambda_4 = l\,\Delta t/h$, so as $\alpha_4 \to 0$, there is no value of $\lambda$ that is independent of $\alpha$ that maintains a reasonable time step. The $\widetilde{Q}_4^{n-1}$ neighborhood contains $\widehat{Q}_4^{n-1}$ and $\widehat{Q}_9^{n-1}$, and $\widehat{Q}_9^{n-1}$ is not contained in any of the other merging neighborhoods, so no other terms can help fix this. This is regardless of the choice of weight $0 < w_{4,0} < 1$.

Using the definition (A.2) with $i = 4$ and $j = 0$, the formula for $\widetilde{Q}_4^{n-1}$ is

$$\widetilde{Q}_4^{n-1} = \frac{1}{1 - w_{4,0}}\,(w_{4,4}\widehat{Q}_4^{n-1} + w_{4,9}\widehat{Q}_9^{n-1}).$$

The $\widetilde{Q}_4^{n-1}$ neighborhood contains $\widehat{Q}_4^{n-1}$ and $\widehat{Q}_9^{n-1}$, and $\widehat{Q}_9^{n-1}$ is not contained in any of the other merging neighborhoods. Using the definition (A.2) with $i = 4$ and $j = 0$, the formula for $\widetilde{Q}_4^{n-1}$ is

$$\widetilde{Q}_4^{n-1} = \frac{1}{1 - w_{4,0}}\,(w_{4,4}\widehat{Q}_4^{n-1} + w_{4,9}\widehat{Q}_9^{n-1}).$$

Setting $w_{4,0}$ to zero reduces to the previous $2 \times 2$ case. Setting $w_{4,0} = 1$ also doesn't work since it would be incompatible with other $3 \times 3$ merging neighborhoods. Thus the multiplier of $\widehat{Q}_9^{n-1}$ is negative, and the scheme is not monotone.■

**SM3. Monotonicity for 45° Ramp, Overlap Count 3.** To finish, we look at a new configuration that has an overlap count of 3.

**Property 6:** For the 45° ramp angle, consider the configuration in Figure SM2 where one small cell merges upward, and another merges to the left, giving cell 1 an overlap count of 3. Weighted SRD results in a monotone scheme for a slightly smaller CFL $\leq 0.92$ on the base grid and the weights:

$$\begin{aligned}
w_{0,0} &= w_{4,4} = 1 \\
w_{1,0}, w_{1,4} &= 1/2 - \alpha_0 \\
w_{1,1} &= 2\alpha_0.
\end{aligned} \tag{SM3.1}$$

The weights in (SM3.1) are those given in (4.2) using $N_1 = 3$, $N_0, N_4 = 1$ and $\alpha_{\text{target}} = 1/2$.

For the $\widehat{Q}_0^n$ update, the update in (A.8) still applies, but we have to examine the quadratic coefficient in front of $\widehat{Q}_0^{n-1}$ more carefully to find when it is positive.

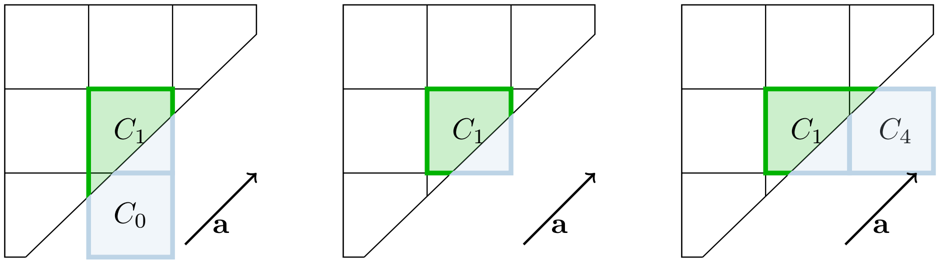


Fig. SM2. *Cell 1 could be in 3 neighborhoods in this 45 degree planar boundary case. Cell 0 merges north, cell 1 is its own neighborhood, and cell 4 merges west. This results in different weights and a slightly smaller CFL for monotonicity than the overlap 2 case in Figure* 3*.*

Substituting the parameters from (SM2.1) and writing everything as a function of the edge length $l$ again transforms the quadratic into a polynomial in the edge length. Writing the CFL limit $\lambda = 2\Delta t/h$, the plot in Figure SM3 shows the coefficient is positive for $\lambda \leq 0.92$, and dips below zero for $\lambda = 0.93$.

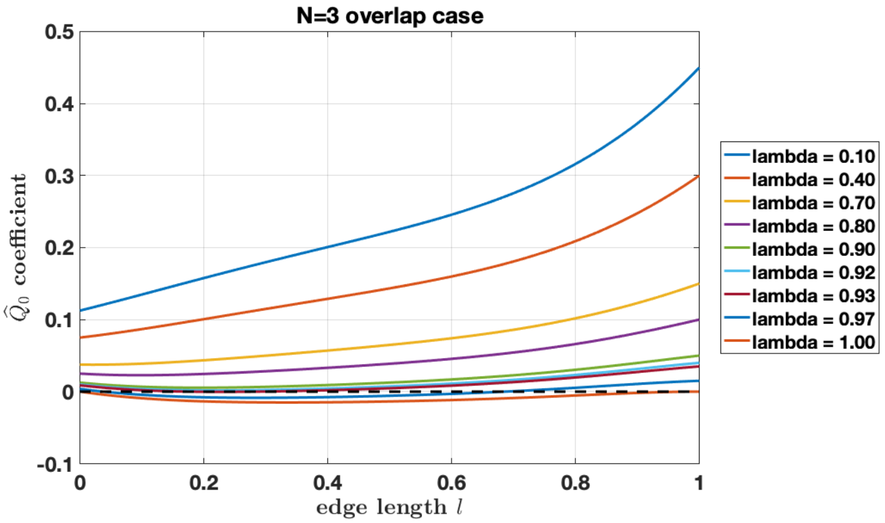


Fig. SM3. *For CFL limit* $\lambda \leq 0.92$ *the positivity of the* $\widehat{Q}_0$ *coefficient is retained.*

Analyzing cell 4 instead of cell 0 results in the same polynomial, after replacing $\alpha_0$ with $\alpha_4$, $\lambda_{1,4} = \lambda_{1,0}$, etc. so cell 4 has positive coefficients with the same slight reduction in the CFL limit too.

Finally, cell 1's update now has more terms than (A.8) since $\widetilde{Q}_1$ is a linear combination of $\widehat{Q}_0$ and $\widehat{Q}_4$. But the only potentially negative coefficient is again the

multiplier in front of $\widehat{Q}_1^{n-1}$, which is exactly the same as in (A.16) and has already been shown to be positive. ■

We have also looked at this configuration with the original weights. It would need a larger reduction down to a CFL $\leq 0.71$ for monotonicity.

*Remark:* Although this configuration does not occur for planar boundaries, the $N = 3$ case does occur for some cells and normal merging in the supersonic vortex mesh in Figure 5, since that example has curved boundaries.

*This manuscript is for review purposes only.*
